# Supplementary material for: GarmentLab: A Unified Simulation and Benchmark for Garment Manipulation
Source: arXiv:2411.01200 source file (2024-12-23)
Supplement: Supplementary file 1 [file supplement.tex]

\documentclass{article}

% if you need to pass options to natbib, use, e.g.:
%     \PassOptionsToPackage{numbers, compress}{natbib}
% before loading neurips_2024

% ready for submission
\usepackage{neurips_2024}
\usepackage{graphicx}
\usepackage{booktabs}
\usepackage{pifont}

% to compile a preprint version, e.g., for submission to arXiv, add add the
% [preprint] option:
%     \usepackage[preprint]{neurips_2024}

% to compile a camera-ready version, add the [final] option, e.g.:
%     \usepackage[final]{neurips_2024}

% to avoid loading the natbib package, add option nonatbib:
%    \usepackage[nonatbib]{neurips_2024}

\usepackage[utf8]{inputenc} % allow utf-8 input
\usepackage[T1]{fontenc}    % use 8-bit T1 fonts
\usepackage{hyperref}       % hyperlinks
\usepackage{url}            % simple URL typesetting
\usepackage{booktabs}       % professional-quality tables
\usepackage{amsfonts}       % blackboard math symbols
\usepackage{nicefrac}       % compact symbols for 1/2, etc.
\usepackage{microtype}      % microtypography
\usepackage{xcolor}         % colors
\usepackage{pifont}
\usepackage{graphicx}
\usepackage{multirow}
\usepackage{threeparttable}
\usepackage{enumitem}
\usepackage{wrapfig}
\title{Supplementary Materials for UniGarment}

\author{%
  David S.~Hippocampus\thanks{Use footnote for providings further information
    about author (webpage, alternative address)---\emph{not} for acknowledging
    funding agencies.} \\
  Department of Computer Science\\
  Cranberry-Lemon University\\
  Pittsburgh, PA 15213 \\
  \texttt{hippo@cs.cranberry-lemon.edu} \\ 
}

\begin{document}

\maketitle

\appendix
\input{supp_tex/supp_overview}
\input{supp_tex/supp_related}
\input{supp_tex/supp_physics}
\input{supp_tex/supp_realbench}
\input{supp_tex/supp_moveit}
\input{supp_tex/supp_teleop}
\input{supp_tex/supp_environment}
\input{supp_tex/supp_limitation}
\input{supp_tex/supp_impact}

\bibliographystyle{plain}
\bibliography{reference}

\end{document}
